# Supplementary material for: Classifying Copy Number Variations Using State Space Modeling of Targeted Sequencing Data: A Case Study in Thalassemia
Source: arXiv:2504.10338 source file (2025-04-14)
Supplement: Supplementary file 1 [file appendix.tex]

\section*{Appendix}

\subsection*{State Space Algorithms}

\subsection*{Parameter Sensitivity}

Here we evaluate the sensitivity of the model to parameter choices. 
A potential criticism of the model defined in \eqref{eq:state_space_model} is its reliance on predefined values for $b$, $\sigma^2$, and $p$. One principled method to address this is to maximize $\mathcal{L}(b, \sigma^2, p) = \log p(y | b, \sigma^2, p)$, requiring integrating out the unobserved values of $x$. However, this approach presents two significant challenges. First, it requires a substantial number of samples for $\mathcal{L}(b, \sigma^2, p)$ to be stable. Second, without an analytic expression for $\mathcal{L}(b, \sigma^2, p)$, standard optimization methods \citep{humpherys2020foundations} cannot be applied. Although alternatives like Bayesian optimization exist \citep{frazier2018tutorial}, they are complex, cumbersome, and bring additional challenges \citep{bengio2017deep}. Furthermore, even if these parameters were optimized, they would likely need to be recalibrated for each specific batch due to variability in factors like operator, reagent age, and equipment. This would necessitate separate parameter estimation for each lab or clinic, rendering the approach commercially impractical.

Instead, we will take an alternative approach and show that the inferred copy ratio is robust to the parameter values chosen over a wide range. Hence, as long as the operator chose ``reasonable'' values for $p$, $b$, and $\sigma^2$,the inferred values will be close to the optimal estimates obtained by the true values. Hence, we perform a sensitivity analysis varying each of the parameters over a range of feasible values and evaluating the mean squared error on the data above. Once again, this is repeated 10 times in order to obtain confidence intervals for each of the values. The results are shown in Figure \ref{fig2}. We find that provided that $p$ and $\sigma^2$ are not set to arbitrarily small values, their effect on CNV estimates is negligible. Only $b$ requires balancing, as it controls how informative each amplicon is on the CNV estimate. However, the reasonable range of $.1$ to $.3$ results in minimal changes in MSE, which coincides with the noise values observed in our data, some of which is plotted in Figure \ref{fig2}. 

\begin{figure}[h]
\centering
\includegraphics[width=1.0\textwidth]{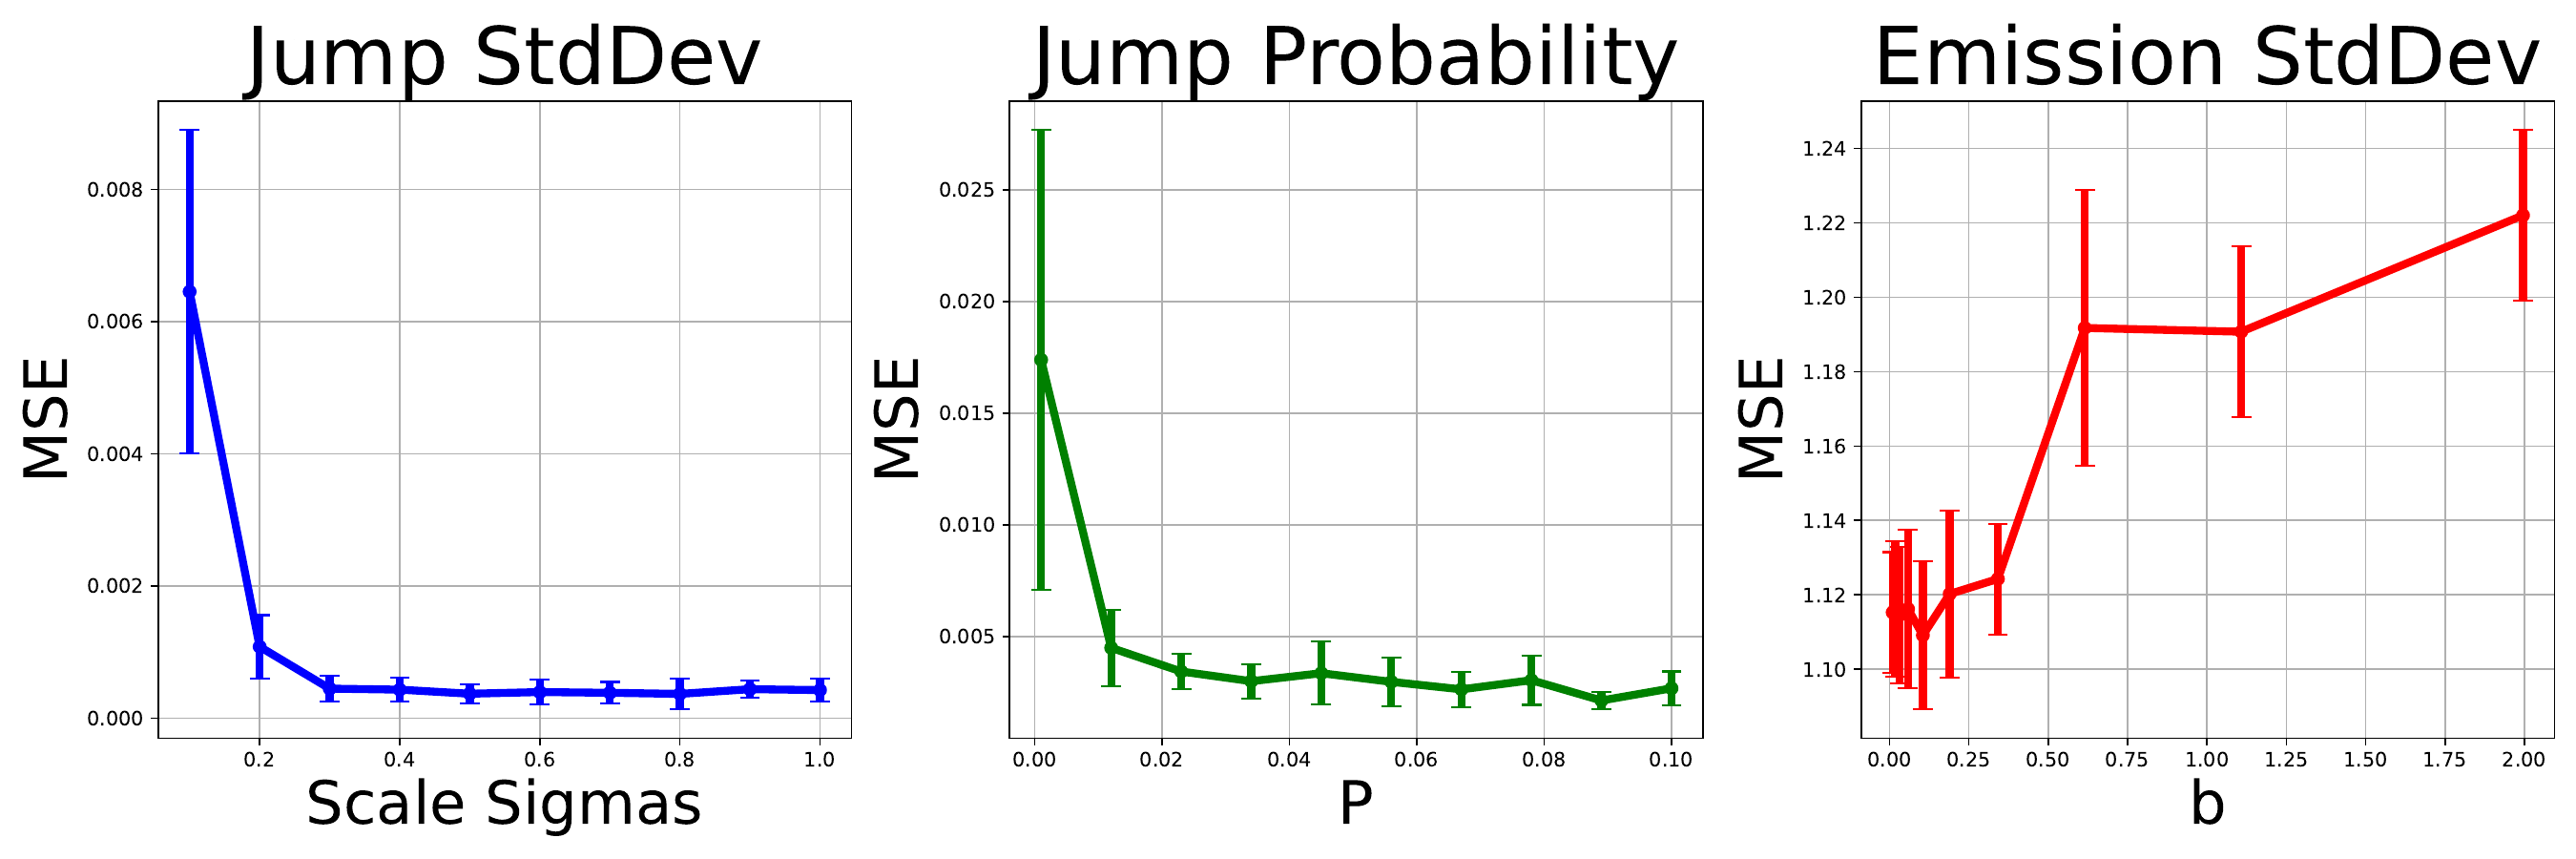}
\caption{The left figure shows the effect that $\sigma^2$ has on the MSE of the estimated CNRs. We can see that setting this parameter to incredibly small values results in a large MSE due to missing true changes. However, beyond $0.4$, the specific value is irrelevant to predictive quality. Likewise, modifying $p$, as shown in the middle plot, results in an inflated MSE for small values, but beyond $0.02$, the specific value has a minimal impact on the MSE. Finally, the parameter $b$ has a ``sweet spot'' of $0.1$; values too small result in overfitting the trajectory, while too large of values result in no information being incorporated. However, around this optimal value there is a wide range where specific valeus have minimal impact on the quality of fit.}\label{fig2}
\end{figure}
